# Supplementary material for: Image Cropping under Design Constraints
Source: arXiv:2310.08892 source file (2023-10-13)
Supplement: Supplementary file 1 [file appendix_prev.tex]

\appendix

\section{Heatmap-based Approach: Model Architecture}
\begin{figure*}[tbh]
\centering
%\fbox{\rule{0pt}{2in} \rule{0.9\linewidth}{0pt}}
\includegraphics[width=.9\linewidth]{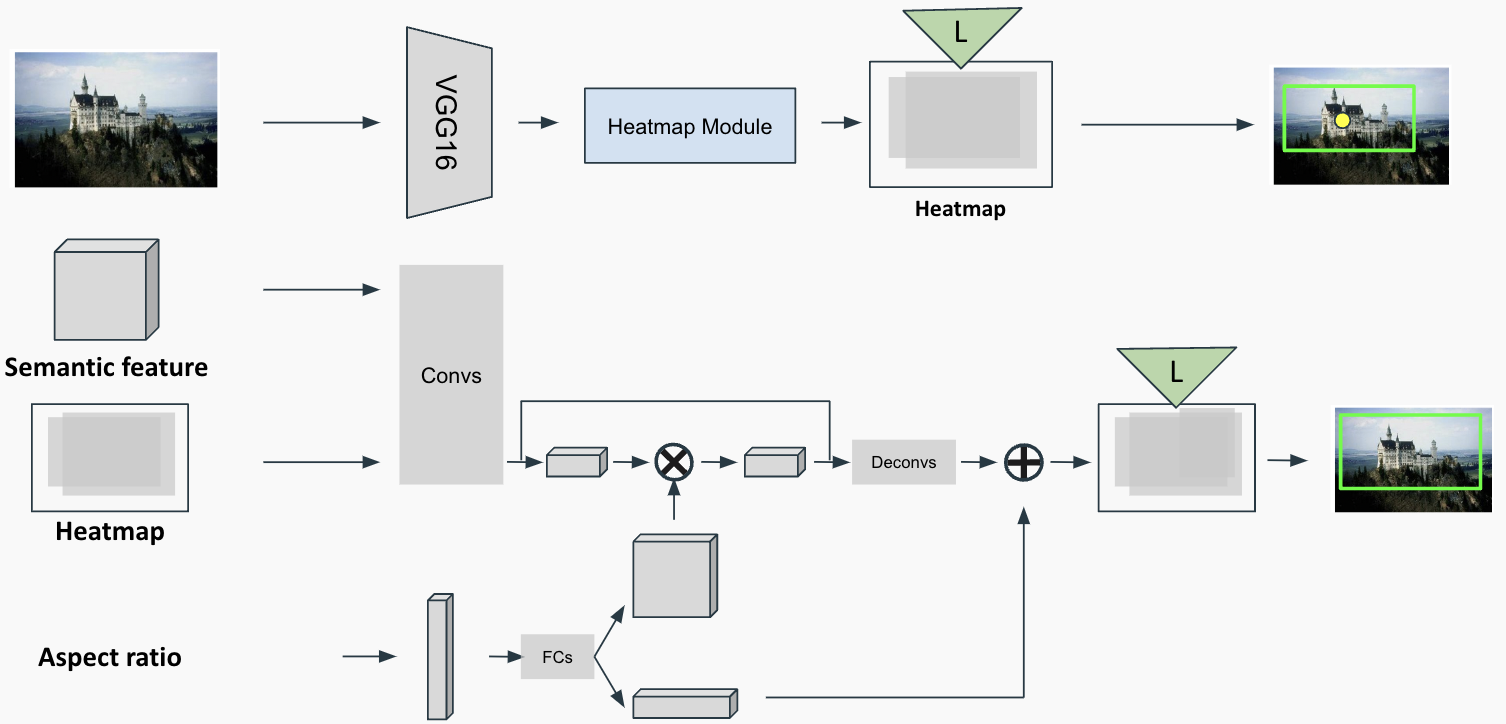}
\caption{手法の詳細}
\label{fig:model_detail}
\end{figure*}

\section{Heatmap Generation for Train Dataset}
\begin{figure*}[tbh]
\centering
%\fbox{\rule{0pt}{2in} \rule{0.9\linewidth}{0pt}}
\includegraphics[width=.9\linewidth]{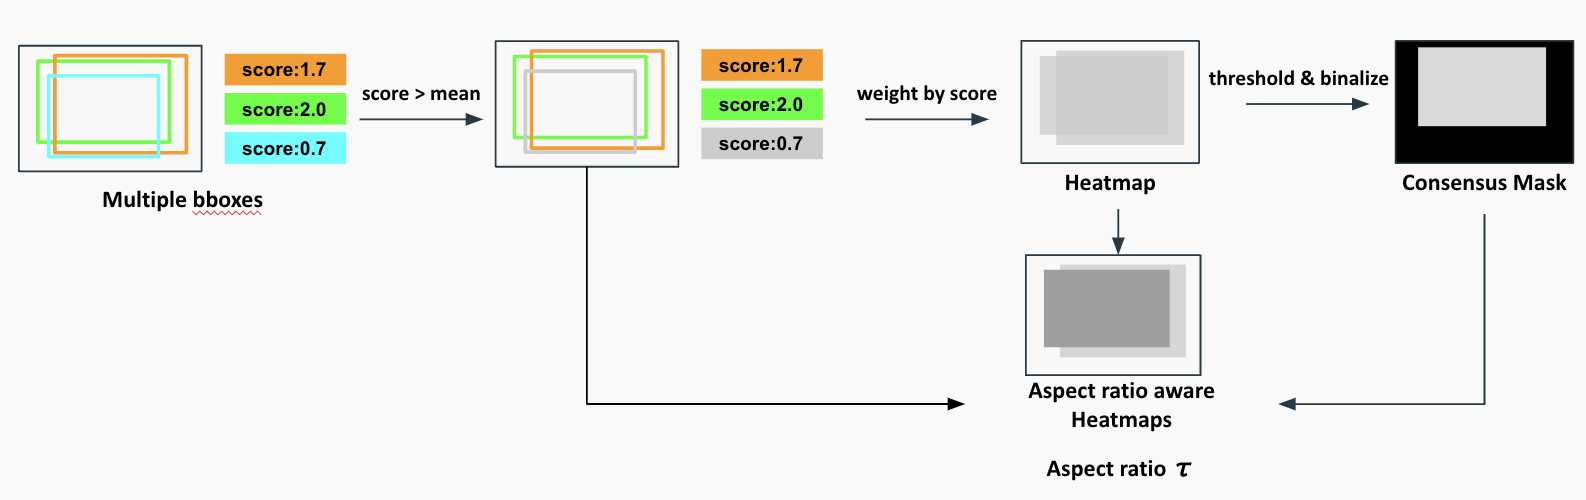}
\caption{学習用のヒートマップ作成方法}
\label{fig:model_detail}
\end{figure*}

\section{Comparison with state of the art}
Without additional constraints, the cropping accuracy of the proposed heatmap-based method was compared to various existing methods. For evaluating the proposed model under no constraints, we use FCDB ~\cite{chen2017quantitative} and FLMS~\cite{fang2014automatic}. 

As illustrated in Table.\ref{tab:eval_IoU}, the aesthetic heatmap-based cropping technique in the proposed method outperforms several existing methods (DIC, A2RL, GAICv1) across both datasets.
A comparison with GAICv2, integrated into the proposed proposal-based method, reveals comparable results. 
While the aesthetics heatmap-based cropping method falls behind CACNET in accuracy without additional constraints, CACNET's output is deemed unsuitable for the context of this study due to its exclusive focus on vertex information for rectangular regions and the presence of other additional constraints.

\begin{table}[t]
\centering
\caption{Results. Comparison of each method with IoU. The results show similar accuracy compared to recent methods.}
\begin{tabular}{l|cc}
\toprule
model  & FCDB~\cite{chen2017quantitative} & FLMS~\cite{fang2014automatic}\\ \midrule
Fang et al. ~\cite{fang2014automatic} &  -         & 0.740\\
DIC~\cite{wang2018deep}    & 0.650          & 0.810          \\
A2-RL~\cite{li2018a2}    & 0.664          & 0.821          \\
VPN~\cite{wei2018good}     & 0.711          &  0.835              \\
GAICv1~\cite{zeng2019reliable} & 0.674               & 0.834               \\
GAICv2~\cite{zeng2020cropping}  & 0.673          &  0.836         \\
CACNET~\cite{Hong_2021_CVPR}   & 0.718 & 0.854 \\ \midrule
Heatmap-based approach         & 0.682          & 0.834  \\\bottomrule
\end{tabular}
\label{tab:eval_IoU}
\end{table}

\section{Comparison on aspect ratio aware image cropping}
Table.\ref{tab:aspect_ratio} shows the results when the aspect ratio of the correct bbox is added as a constraint. The prepared heatmap-based method shows results comparable to the SOTA model. heatmap-based shows lower values compared to Mars~\cite{li2020learning}, but the latter outputs cropping regions using images as input and thus uses more informative features compared to the proposed method. The latter uses images as input and outputs cropping regions, so it uses features that are more informative than the proposed method. The prepared heatmap-based method uses a heatmap as an intermediate representation in the input and shows comparable results to the other methods, despite the smaller information content of the input compared to the other methods.

\begin{table}[tbh]
\centering
\caption{Results with aspect ratio condition (FCDB ~\cite{chen2017quantitative}).}
\begin{tabular}{l|c}
\toprule
model                 & IoU   \\ \midrule
VPN~\cite{wei2018good}     & 0.716 \\
GAICv2~\cite{zeng2020cropping}  & 0.673 \\
CACNet~\cite{Hong_2021_CVPR} & 0.718 \\
Mars~\cite{li2020learning}     & 0.736 \\ \midrule 
Heatmap-based                   & 0.784? \\ \bottomrule
\end{tabular}
\label{tab:aspect_ratio}
\end{table}

\section{Application}
%広告バナー生成
The method proposed in this study holds potential for integration into the automation of advertisement image generation. In the conventional process of manually creating advertising materials, images are chosen from a stock and then modified to fit the required aspect ratio for the target media while incorporating the intended message. This procedure must be carried out multiple times to produce a range of candidates, ultimately leading to advertising materials that meet user expectations. By implementing the techniques proposed in this study, it is possible to automatically generate advertising materials, as illustrated in Figure 6, without human intervention. This approach alleviates the burden of creating ad materials and allows users to focus on selecting the most effective options from the generated materials.

\section{Limitations}
\paragraph{\textbf{Running Speed.}}
Heatmap-based methods use an optimization approach that iteratively evaluates scores, so there is a tradeoff between accuracy and speed of inferencing. Therefore, the inference speed of the proposed method is slower than the proposal-based and baseline methods. However, it is suggested that by reducing the number of refinements by increasing the step size, as shown in Figure 5, it is possible to ensure inference speed without much loss of accuracy.

\paragraph{\textbf{Layout specification.}}
The method proposed in this paper can specify "areas to be left" from the image before cropping. However, since it is not possible to specify "areas to be reserved" in the cropped area, it may not be possible to obtain images with the desired layout. As a means of solving such a case, it is thought that the problem can be handled by separately specifying particularly important areas in the cropped image and scoring the overlap ratio with the layout mask.

\section{Optimization algorithm}

%制約を加味した処理をする。
By applying a constraint-weighted process on $h^{c}$, we obtain the cropping result $crop$ corresponding to Condition $\mathcal{C}$. In multi-conditioned cropping, the crop can be determined by three variables:~,~,~.

% \begin{algorithm}
% \caption{Bounding box optimization}
% \label{alg1}
% \begin{algorithmic}[1]
% \Require{$h_c$:conditioned heatmap,$l$:spatial layout,$\tau$:aspect ratio}
% \Function {Optimization}{$h_c$,$l$,$\tau$,$n$}
%     \State{$\alpha \gets 10000$}
%     \State{$best\_score \gets 0$}
%     \State{$N \gets n$} \Comment{iteration}
%     \While{$N \neq 0$}
%         \State{$crop \gets Cropping(\tau)$}
%         \State{$score_{h} \gets Calculate\_heatmap\_score(h_c, crop)$}
%         \State{$score_{l} \gets Calculate\_recall(l, crop)$}
%         \State{$Score = score_{h} + \alpha \times score_{l}$}
%         \If{$Score > Best\_score$}
%             \State{$best\_crop \gets crop$}
%         \EndIf
%         \State $N \gets N - 1$
%     \EndWhile
% \State \Return{best\_crop}
% \EndFunction
% \end{algorithmic}
% \end{algorithm}

\section{Inference　algorithm}

\begin{algorithm}
\caption{Image cropping from multi-conditioned heatmap}
\label{alg2}
\begin{algorithmic}[1]
\Function {Cropping}{$\tau$}
    \State{$x_1 \gets \{0,width/2\}$}
    \State{$y_1 \gets \{0,height/2\}$}
    \State{$x\_lim = width - x_1, y\_lim = height - y_1$}
    \State{$\tau_{rest} = y\_lim/x\_lim$}
    \If{$(\tau_{rest} >=1) \And (\tau_{rest} <= \tau)$}
    \State{$s \gets 0$ to $y\_lim$ step $p$ } 
        \If{$\tau <= 1$}
        \State{$x2 = x_1 + s * \tau$}
        \Else
        \State{$x2 = x_1 + s / \tau$}
        \EndIf
        \State{$y2 = y_1 + s$}
    \EndIf
    \If{$(\tau_{rest} >=1) \And (\tau_{rest} > \tau)$}
        \State{$s \gets \{0, x\_lim \}$}
        \State{$x2 = x_1 + s$}
        \State{$y2 = y_1 + s * \tau$}
    \EndIf 
   \If{$(\tau_{rest} <1) \And (\tau_{rest} <= \tau)$}
        \State{$s \gets 0$ to $y\_lim$ step $p$ } 
        \State{$x2 = x_1 + s / \tau$}
        \State{$y2 = y_1 + s$}
    \EndIf
    \If{$(\tau_{rest} <1) \And (\tau_{rest} > \tau)$}
        \State{$s \gets 0$ to $x\_lim$ step $p$ }
        \State{$x2 = x_1 + s$}
        \If{$\tau <= 1$}
            \State{$y2 = y_1 + s * \tau$} 
        \Else{}
            \State{$y2 = y_1 + s / \tau $}
        \EndIf
    \EndIf\\
    \Return $[x1,x2,y1,y2]$
    \EndFunction
\end{algorithmic}
\end{algorithm}

\begin{comment}
\section{Evaluation Datasets}

\begin{figure*}[h]
\centering
%\fbox{\rule{0pt}{2in} \rule{0.9\linewidth}{0pt}}
\includegraphics[width=.9\linewidth]{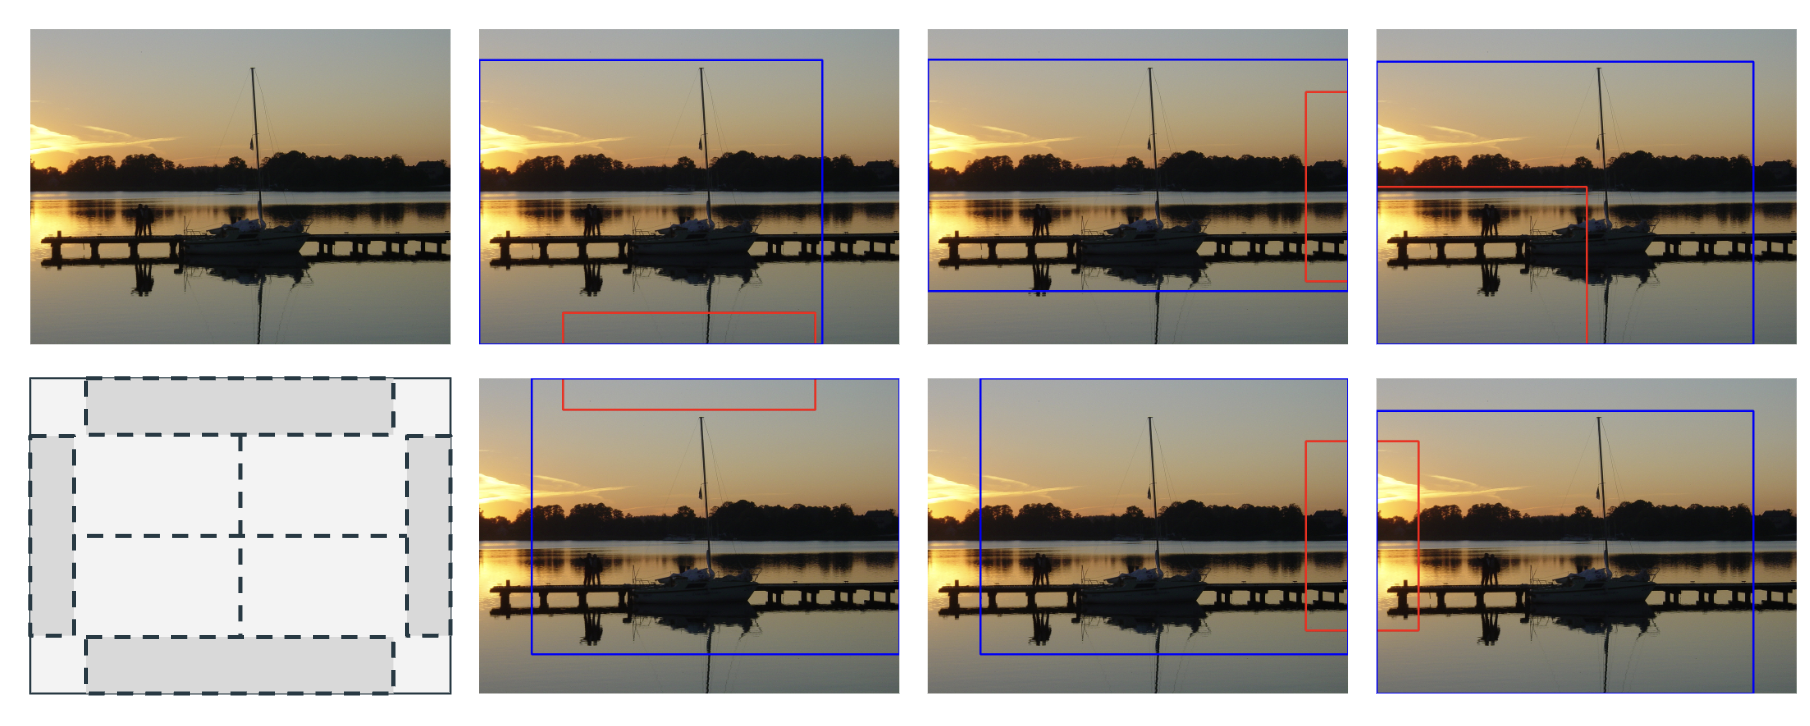}
\caption{Example of evaluation dataset. The upper left shows the original image and the lower left represents the specified blank area. The blue boxes on the other images indicate the ground truth region as aesthetic cropping, and the red boxes indicate the user-defined spatial layout.}
\label{fig:example_dataset}
\end{figure*}

\end{comment}
